# Supplementary material for: Remote effects spatial process models for modeling teleconnections
Source: arXiv:1612.06303 source file (2018-07-02)
Supplement: Supplementary file 1 [file geostat_telecon_supplement-concordance.tex]

\Sconcordance{concordance:geostat_telecon_supplement.tex:geostat_telecon_supplement.Rnw:%
1 114 1 48 0 1 5 1 1 1 17 1 1 1 80 384 1 1 29 85 1 1 25 49 1 1 4 %
12 1 1 8 2 1 1 14 12 1 1 27 11 1 5 0 10 1}
